# Supplementary material for: Agent Workflow Memory
Source: arXiv:2409.07429 source file (2024-09-11)
Supplement: Supplementary file 1 [file results_deprecated.tex]

\section{Experiments}
\label{sec:4:experiments}

In this section, we first introduce the two major benchmarks ---WebArena and Mind2Web, and top-performing baselines on them (\S\ref{sec:4.1:benchmark-and-baseline}). Next, we present our \awm approach on both benchmarks, showcasing its ability to achieve task success and generalization across varied setups (\S\ref{sec:4.2:webarena-results}, \S\ref{sec:4.3:mind2web-results}).


%%%%%%%%%%%%%%%%%%%%%%%%%%%%%%%%%%%%%%%%%%%%%%%%%%%%%
\subsection{Benchmarks and Baselines}
\label{sec:4.1:benchmark-and-baseline}

\paragraph{WebArena}
% dataset
\citep{zhou2024webarena} provides 812 web navigation tasks on five websites that cover four common application domains: e-commerce, social forum discussions, collaborative software development, and content management. Most importantly, WebArena supports rigorous evaluation on the functional correctness of agent trajectories. 

% sota method
We adopt the current state-of-the-art method without human-distilled knowledge, BrowserGym \citep{drouin2024workarena}, which altered the agent action space to a set of bid-based actions. We adopt the BrowserGym framework alone with its bid-based action space, and represent webpages using accessibility trees, aligning to the environment representation in \citet{zhou2024webarena}. Because BrowserGym inputs both webpage HTML and accessibility tree representations, to keep a fair comparison with our method, we also run the BrowserGym version with only accessibility tree webpage representations, denoted as BrowserGym$_{\it ax-tree}$.
%
Note that, the SteP \citep{sodhi2023heap} method outperforms BrowserGym, yet achieves so by adding 14 human expert written workflows tailored for solving WebArena. We thus view SteP as an oracle setting and will show \awm's superior results over it.


% atm setup
Aligning with baseline approaches, we use \texttt{gpt-4} and use a temperature of $0.0$ to ensure fairly stable model outputs.
Because WebArena only contains test examples and no additional high-quality, domain-aligned examples exist, we only conduct \awm in the online setting as introduced in \S\ref{sec:3.3.2:online}.
 


\paragraph{Mind2Web}
\citep{deng2023mindweb} features web navigation tasks across a wide range of websites and domains, stressing the generalization abilities of agents over versatile operations and environments. 
Each task in Mind2Web has a fixed number of steps; at each step, the agent needs to predict an action, which is evaluated in three dimensions: (1) \textit{Element accuracy}: to check if the correct element is selected in the predicted action, (2) \textit{Action F$_1$} to check if the action taken is correct, and aggregating (1) and (2) yields, (3) \textit{Step success rate} to check if both element and action selection is correct at the current step. Lastly, after completing every step in the given task, the last metric (4) \textit{success rate} measures if all intermediate steps are successfully conducted for this task, \ie, only when all steps score 1 in metric (3) get a full score in metric (4).

Because Mind2Web provides a training set covering a portion of tested websites and domains, we explore both \textit{offline} setting that induces workflows from the training set and applies to test sets, as well as the \textit{online} setting, where we do streaming induction and inference on test queries only.

Since we focus on LM-based agents that only take textual inputs, we compare \awm to two state-of-the-art methods, MindAct \citep{deng2023mindweb} and Synapse \citep{zheng2024synapse}. MindAct introduces webpage element filtering and multi-choice task format to ease observation processing, and Synapse changes the format to a trajectory style and augments retrieved relevant examples. We integrate the element filtering adopted in both methods, and added workflows instead of retrieved examples in Synapse, to verify the superiority of reusable workflows over concrete examples. To fairly compare with all baseline methods, we run \awm with both \texttt{gpt-3.5-turbo} and \texttt{gpt-4} models.

For both datasets, we induce and incorporate workflows on a website basis. In other words, we group examples by their associated websites, and respectively run \awm on each group. We report the micro-average scores over all groups, \ie, average scores of all examples. This mechanism maintains an effectively small workflow repository, while bringing the maximum benefit to the pertinent tasks.


\input{sections/results/webarena}
\input{sections/results/mind2web}
